# Supplementary material for: Hardness of Graph-Structured Algebraic and Symbolic Problems
Source: arXiv:2109.12736 source file (2022-11-08)
Supplement: Supplementary file 1 [file appendix_schur.tex]

\begin{proof}

Proof for Item \ref{itm:series}: Define 

$$\series(\mL, \mU)\defeq\left[
\begin{array}{ccccc}
\mL_{1, 1}& 0&  \mL_{1, 2}&\mL_{[1, [3,n]]}& \vzero \\
0&\mU_{1, 1}&\mU_{1, 2}&\vzero & \mU_{[1, [3, m]]}\\
\mL_{2, 1}&\mU_{2, 1} & \mL_{2, 2}+\mU_{2, 2} & \mL_{[2, [3,n]]} &\mU_{[2, [3, m]]} \\
\mL_{[[3,n], 1]}& \vzero &  \mL_{[[3,n], 2]} & \mL_{[[3, n], [3, n]]} & \vzero\\
\vzero& \mU_{[[3, m], 1]} & \mU_{[[3, m], 2]} & \vzero & \mU_{[[3, m], [3, m]]} \\

\end{array}\right].$$ Let $T=\{1, 2, 3\}, F=\{4, \ldots, n+m-2\}$. $\size(\series(\mL, \mU))\le \size(\mL)+\size(\mU)$ is satisfied
because $\size(\mA)+\size(\mB)\ge \size(\mA+\mB)$ for any matrices $\mA, \mB$ over $\mathbb{Z}_p$. By definition, we have  
\begin{align*}
    &\sc(\series(\mL, \mU), \{1, 2, 3\})\\
    =& (\series(\mL, \mU))_{[T, T]}-\series(\mL, \mU)_{[T, F]}
    \series(\mL, \mU)_{[F, F]}^{-1}
    \series(\mL, \mU)_{[F, T]}\\
    =&\left[\begin{array}{ccc}\mL_{1, 1} & 0  & \mL_{1, 2}\\ 0 & \mU_{1, 1} & \mU_{1, 2} \\ \mL_{2, 1} & \mU_{2, 1} & \mL_{2, 2} + \mU_{2, 2}\end{array}\right]\\
    &-\left[\begin{array}{cc}\mL_{[1, [3,n]]}& \vzero \\\vzero & \mU_{[1, [3, m]]} \\  \mL_{[2, [3,n]]} &\mU_{[2, [3, m]]} \end{array}\right]
    \left[\begin{array}{cc}\mL_{[[3, n], [3, n]]} & \vzero\\
\vzero & \mU_{[[3, m], [3, m]]} \end{array}\right]^{-1}
    \left[\begin{array}{ccc}\mL_{[[3,n], 1]}& 0& \mL_{[[3,n], 2]}\\ 0& \mU_{[[3, m], 1]}&\mU_{[[3, m], 2]}\end{array}\right]\\
    =&\left[\begin{array}{ccc}\mL_{1, 1} & 0  & \mL_{1, 2}\\ 0 & \mU_{1, 1} & \mU_{1, 2} \\ \mL_{2, 1} & \mU_{2, 1} & \mL_{2, 2} + \mU_{2, 2}\end{array}\right]\\
    &-\left[\begin{array}{ccc}\mL_{[1, [3,n]]}\mL_{[[3, n], [3, n]]}^{-1} \mL_{[[3,n], 1]} & \vzero & \mL_{[1, [3,n]]}\mL_{[[3, n], [3, n]]}^{-1} \mL_{[[3,n], 2]}\\
    \vzero & \mU_{[1, [3,m]]}\mU_{[[3, m], [3, m]]}^{-1} \mU_{[[3,m], 1]} & \mU_{[1, [3,m]]}\mU_{[[3, m], [3, m]]}^{-1} \mU_{[[3,m], 2]}\\
    \mL_{[2, [3,n]]}\mL_{[[3, n], [3, n]]}^{-1} \mL_{[[3,n], 1]} & \mU_{[2, [3,m]]}\mU_{[[3, m], [3, m]]}^{-1} \mU_{[[3,m], 1]} & \left(\makecell{\mL_{[2, [3,n]]}\mL_{[[3, n], [3, n]]}^{-1} \mL_{[[3,n], 2]}\\+\mU_{[2, [3,m]]}\mU_{[[3, m], [3, m]]}^{-1} \mU_{[[3,m], 2]}}\right)
    \end{array}\right]\\
    =&\left[\begin{array}{ccc}\sc(\mL, \{1, 2\})_{1, 1} & 0 & \sc(\mL, \{1, 2\})_{1, 2}\\ 0 &\sc(\mU, \{1, 2\})_{1, 1} & \sc(\mU, \{1, 2\})_{1, 2}\\ \sc(\mL, \{1, 2\})_{2, 1}  & \sc(\mU, \{1, 2\})_{2, 1} & \sc(\mL, \{1, 2\})_{2, 2}+\sc(\mU, \{1, 2\})_{2, 2}\end{array}\right]\\
    =&\left[\begin{array}{ccc}a^{-1} & 0 & -a^{-1}\\ 0 &b^{-1} & -b^{-1}\\ -a^{-1}  & -b^{-1} & a^{-1}+b^{-1}\end{array}\right].
\end{align*} By Lemma \ref{lem:commutative}, 
\begin{align*}
    &\sc(\series(\mL, \mU), \{1, 2\})\\
    =&\sc(\sc(\series(\mL, \mU), \{1, 2, 3\}), \{1, 2\})\\
    =&\sc\left(\left[\begin{array}{ccc}a^{-1} & 0 & -a^{-1}\\ 0 &b^{-1} & -b^{-1}\\ -a^{-1}  & -b^{-1} & a^{-1}+b^{-1}\end{array}\right], \{1, 2\}\right)\\
    =&\left[\begin{array}{cc}\frac{1}{a+b} & -\frac{1}{a+b}\\ -\frac{1}{a+b} &\frac{1}{a+b}\end{array}\right].
\end{align*}
Proof for Item \ref{itm:parallel}:
Define 

$$\parallel(\mL, \mU)\defeq \left[
\begin{array}{cccc}
\multicolumn{2}{c}{\multirow{2}{*}{$\mL_{[\{1, 2\}, \{1, 2\}]}+\mU_{[\{1, 2\}, \{1, 2\}]}$}}& \mL_{[1, [3, n]]} & \mU_{[1, [3, m]]} \\
\multicolumn{2}{c}{}& \mL_{[2, [3, n]]}& \mU_{[2, [3, m]]} \\
\mL_{[[3, n], 1]} & \mL_{[[3, n], 2]}  & \mL_{[[3,n], [3,n]]}& \vzero\\
\mU_{[[3, m], 1]} & \mU_{[[3, m], 2]}  & \vzero & \mU_{[[3,m], [3,m]]}
\end{array}\right].$$ $\size(\parallel(\mL, \mU))\le \size(\mL)+\size(\mU)$ is satisfied for the same reason as in Item \ref{itm:series}. Let $T=\{1, 2\}, F=\{3, \ldots, n+m-2\}$. By definition, we have 
\begin{align*}
    &\sc(\parallel(\mL, \mU), \{1, 2\})\\
    =& (\mL+\mU)_{[T, T]}-\parallel(\mL, \mU)_{[T, F]}
    \parallel(\mL, \mU)_{[F, F]}^{-1}
    \parallel(\mL, \mU)_{[F, T]}\\
    =&(\mL+\mU)_{[T, T]}-\left[\begin{array}{cc}\mL_{[1, [3, n]]} & \mU_{[1, [3, m]]}\\ \mL_{[2, [3, n]]}&\mU_{[2, [3, m]]}\end{array}\right]
    \left[\begin{array}{cc}\mL_{[[3, n], [3, n]]} & \vzero \\ \vzero & \mU_{[[3, m], [3, m]]}\end{array}\right]^{-1}
    \left[\begin{array}{cc}\mL_{[[3, n], 1]} & \mL_{[[3, n], 2]}\\\mU_{[[3, m], 1]} & \mU_{[[3, m], 2]}\end{array}\right]\\
    =&(\mL+\mU)_{[T, T]}-\left(\mL_{[\{1, 2\}, [3, n]]} \mL_{[[3, n], [3, n]]}^{-1} \mL_{[[3, n], \{1,2\}]} + \mU_{[\{1, 2\}, [3, m]]} \mU_{[[3, m], [3, m]]}^{-1} \mU_{[[3, m], \{1,2\}]}\right)\\
    =&\sc(\mL, \{1, 2\})+\sc(\mU, \{1, 2\})\\
    =&\vchi_{1, 2}^\top (a^{-1}+b^{-1}) \vchi_{1, 2} \qedhere
\end{align*}
\end{proof}
